# Supplementary material for: Shape My Moves: Text-Driven Shape-Aware Synthesis of Human Motions
Source: arXiv:2504.03639 source file (2025-04-04)
Supplement: Supplementary file 1 [file supp_template.tex]

\begin{table*}[t]
\centering
\caption{\textbf{Template for Shape Description Data Input.} This table provides a structured format for users to input detailed measurements of human body attributes. It includes fields for height, weight, body type, and specific measurements for chest, waist, hips, arms, and legs, ensuring comprehensive data collection for shape-aware motion synthesis.}
\begin{tcolorbox}[colback=gray!8, colframe=black!90, boxrule=1pt, sharp corners]
\begin{enumerate}[leftmargin=*]
    \item A \textless{}gender\textgreater{} standing \textless{}height\textgreater{} cm tall, with a chest circumference of \textless{}chest\textgreater{} cm, waist circumference of \textless{}waist\textgreater{} cm, and hip circumference of \textless{}hip\textgreater{} cm. The length of the arm is \textless{}arm\textgreater{} cm and leg height is \textless{}leg\textgreater{} cm.
    \item This individual, a \textless{}gender\textgreater{}, has a height of \textless{}height\textgreater{} cm. Their body measurements include a chest of \textless{}chest\textgreater{} cm, a waist of \textless{}waist\textgreater{} cm, and hips measuring \textless{}hip\textgreater{} cm. The arm extends \textless{}arm\textgreater{} cm and the legs are \textless{}leg\textgreater{} cm long.
    \item The \textless{}gender\textgreater{} stands \textless{}height\textgreater{} cm tall. They have a chest circumference of \textless{}chest\textgreater{} cm, a waist of \textless{}waist\textgreater{} cm, and hips that measure \textless{}hip\textgreater{} cm. The arm and leg measurements are \textless{}arm\textgreater{} cm and \textless{}leg\textgreater{} cm, respectively.
    \item Describing the \textless{}gender\textgreater{}: They are \textless{}height\textgreater{} cm in height, with body measurements that include a chest of \textless{}chest\textgreater{} cm, a waist of \textless{}waist\textgreater{} cm, and hips of \textless{}hip\textgreater{} cm. Additionally, their arm measures \textless{}arm\textgreater{} cm, and their leg height is \textless{}leg\textgreater{} cm.
    \item Here is a \textless{}gender\textgreater{} with a height of \textless{}height\textgreater{} cm. Their measurements are as follows: chest \textless{}chest\textgreater{} cm, waist \textless{}waist\textgreater{} cm, and hips \textless{}hip\textgreater{} cm. The lengths of the arm and legs are \textless{}arm\textgreater{} cm and \textless{}leg\textgreater{} cm respectively.
    \item You see a \textless{}gender\textgreater{} whose physical stature includes a height of \textless{}height\textgreater{} cm. Notable measurements are a chest circumference of \textless{}chest\textgreater{} cm, waist circumference of \textless{}waist\textgreater{} cm, and hip circumference of \textless{}hip\textgreater{} cm, with an arm length of \textless{}arm\textgreater{} cm and leg height of \textless{}leg\textgreater{} cm.
    \item A \textless{}gender\textgreater{} with these dimensions: \textless{}height\textgreater{} cm tall, chest \textless{}chest\textgreater{} cm, waist \textless{}waist\textgreater{} cm, hips \textless{}hip\textgreater{} cm, arm \textless{}arm\textgreater{} cm, and leg height \textless{}leg\textgreater{} cm.
    \item Consider a \textless{}gender\textgreater{} who is \textless{}height\textgreater{} cm tall. They have a chest of \textless{}chest\textgreater{} cm, waist of \textless{}waist\textgreater{} cm, and hips of \textless{}hip\textgreater{} cm. Their arm is \textless{}arm\textgreater{} cm long, and their legs measure \textless{}leg\textgreater{} cm in height.
    \item Profile of a \textless{}gender\textgreater{}: Height of \textless{}height\textgreater{} cm, with a chest measurement of \textless{}chest\textgreater{} cm, waist of \textless{}waist\textgreater{} cm, and hips spanning \textless{}hip\textgreater{} cm. The arm and leg heights are \textless{}arm\textgreater{} cm and \textless{}leg\textgreater{} cm, respectively.
    \item A detailed look at a \textless{}gender\textgreater{}: They stand \textless{}height\textgreater{} cm tall, and feature a chest of \textless{}chest\textgreater{} cm, a waist of \textless{}waist\textgreater{} cm, and hips measuring \textless{}hip\textgreater{} cm. Their arm length is \textless{}arm\textgreater{} cm, and the leg height is \textless{}leg\textgreater{} cm.
\end{enumerate}
\end{tcolorbox}
\label{tab:supp_template}
\end{table*}
